# Supplementary material for: Unsupervised Monocular Depth Learning in Dynamic Scenes
Source: arXiv:2010.16404 ancillary file (2020-11-07)
Supplement: Supplementary file 1 [file supplementary_material.pdf]

# Supplementary Material

The weights of the losses in Eq. (4-7) in the main paper are the same for all datasets and are summarized in Table 1.

| Coefficient | Value |
|---|---|
| $\alpha_{\text{mot}}$ | 1.0 |
| $\beta_{\text{mot}}$ | 0.2 |
| $\alpha_{\text{dep}}$ | 0.001 |
| $\alpha_{\text{cyc}}$ | 0.001 |
| $\beta_{\text{cyc}}$ | 0.05 |
| $\alpha_{\text{rgb}}$ | 1.0 |
| $\beta_{\text{rgb}}$ | 3.0 |

Table 1: Weights of the various losses, as defined in Eq. (4-7) of the paper.

As additional reference for our regularization techniques, we visualize the effect of the square root norm in Figure 1.

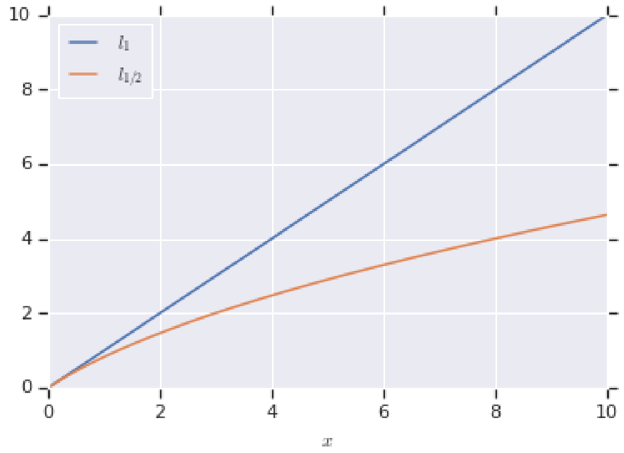


Figure 1: Visualization of the regularizers $l_1(x) \equiv x$ and $l_{1/2}(x) \equiv 2\sqrt{x+1} - 2$. The offset $-2$ is added for a better comparison and doesn't affect the optimization.

In Figures 2 and 3, we visualize depth and 3D motion learned using our unsupervised approach from a collection of YouTube videos and sequences from the Cityscapes dataset. In many of them, there are vehicles and people moving around. The collection of YouTube videos were recorded with hand-held monocular cameras by people walking around in diverse environments, and the camera intrinsics were unknown to us.

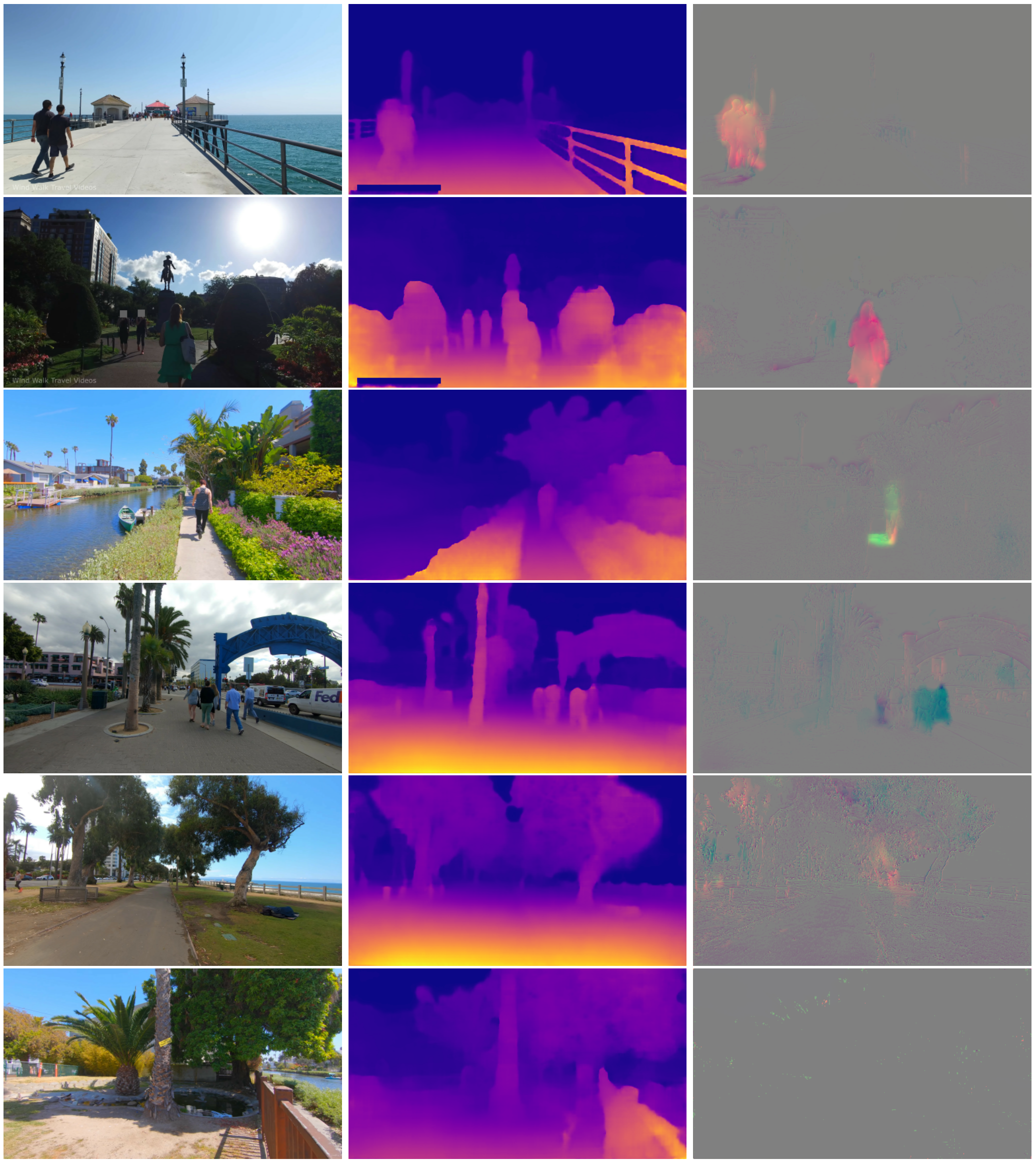

Figure 2: Learned object motion maps (right column) and depth maps (middle column) for RGB frames (left column) from a collection of YouTube videos with moving cameras. The last two examples show static scenes, where the object motion maps are close to zero.

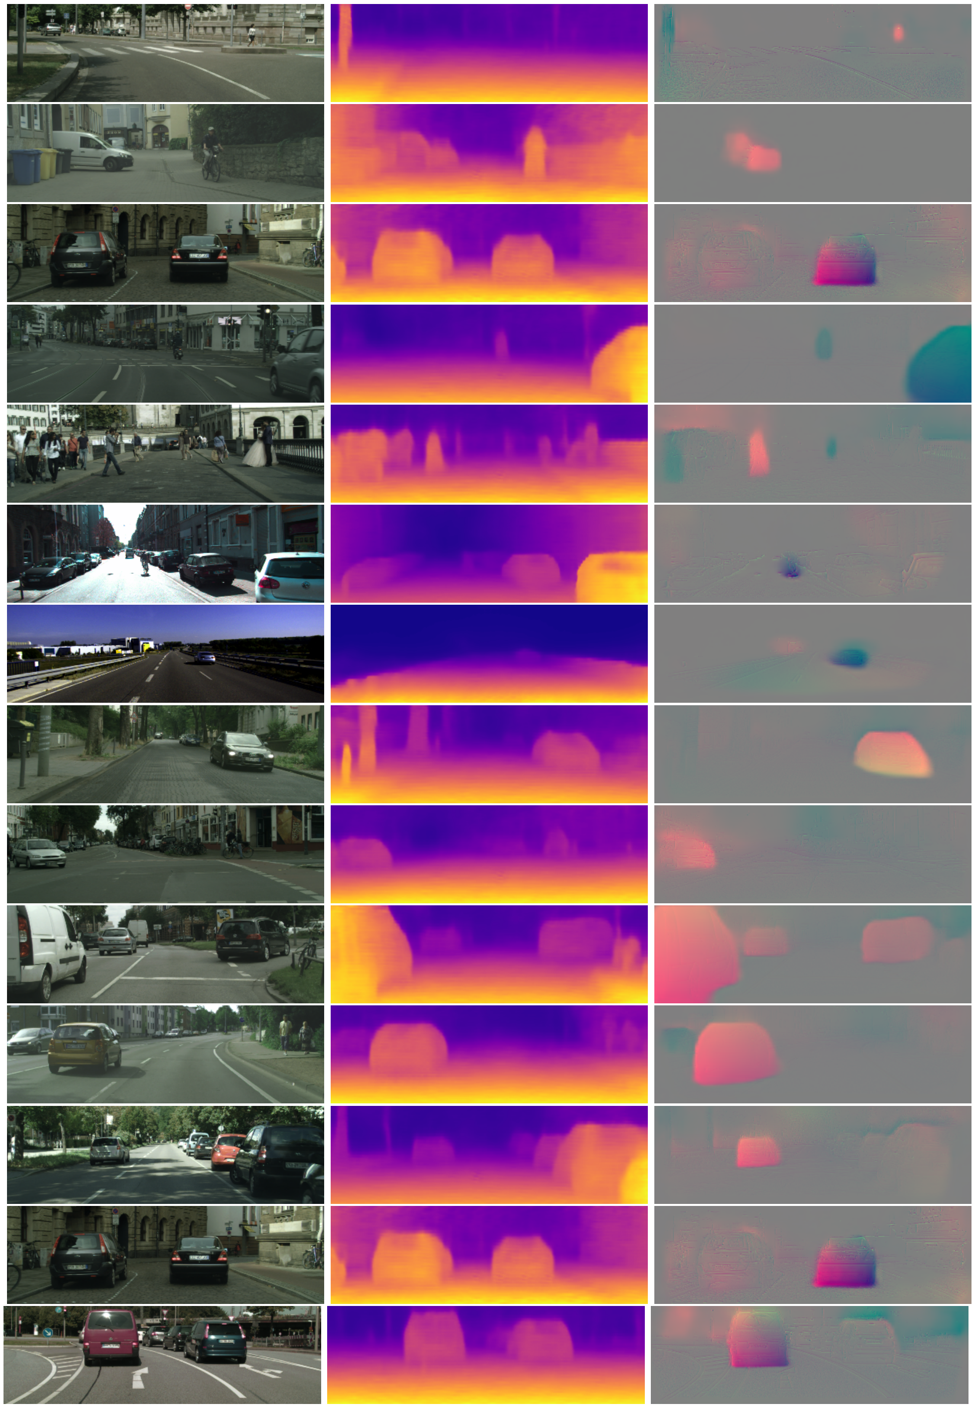

Figure 3: Learned object motion maps (right column) and depth maps (middle column) for RGB frames (left column) from the Cityscapes dataset.

Figure 4 provides another visualization of the learned depth and 3D motion maps on the Waymo Open Dataset. We can more easily observe how the model is able to decompose motion.

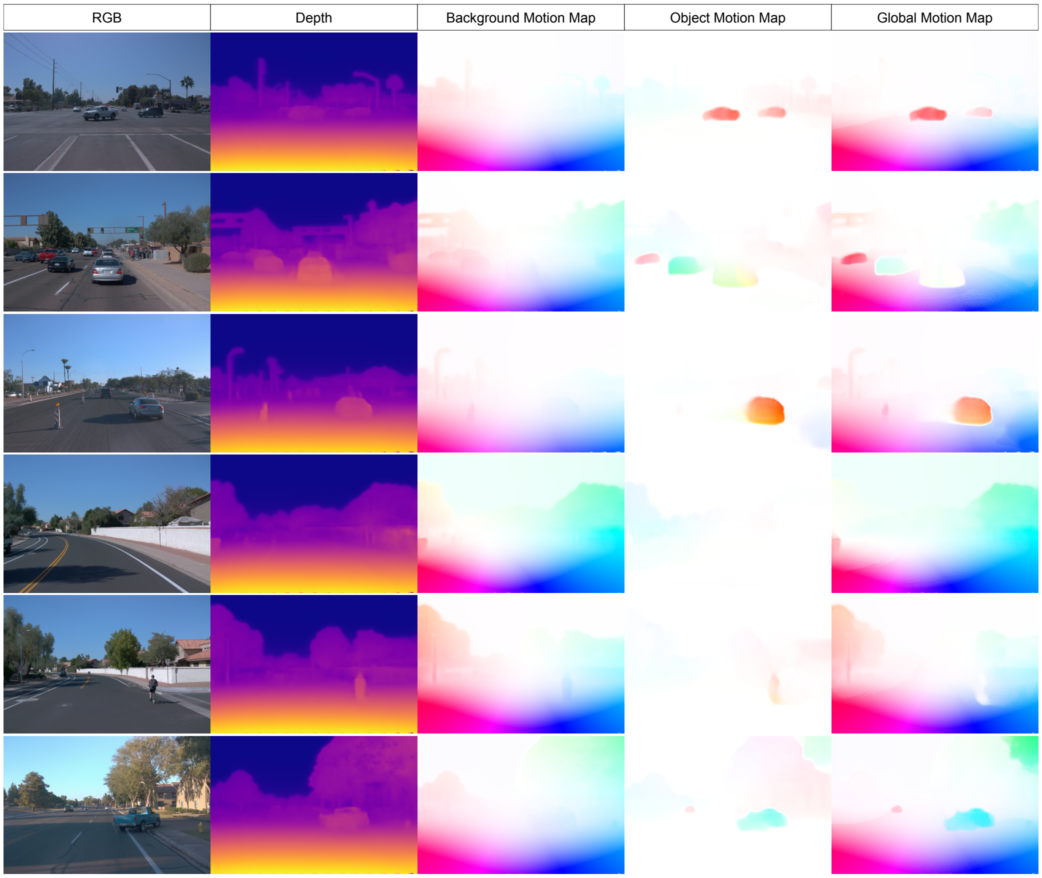


Figure 4: This figure shows RGB images, depth maps, and the 2D-appearance flows projected from 3D motion maps on the Waymo Open Dataset. Here, we colorize based on flow direction with intensity corresponding to flow magnitude. Using our depth and background motion estimate, we can derive 2D appearance flow of static parts of the scene (middle). We can use the same procedure to visualize our object motion field and their global composite (right), respectively.
